# Supplementary material for: Sparse Vicious Attacks on Graph Neural Networks
Source: arXiv:2209.09688 source file (2022-09-20)
Supplement: Supplementary file 2 [file abl_X.tex]

\begin{table}[h!]
\centering
\caption{\label{tab:X}Results under different assumptions for the creation of the vicious nodes feature matrix. While not optimizing for this, SAVAGE is robust under different settings and mainatins strong results.}
\begin{tabular}{@{}lcccc@{}}
\toprule
Method   & AR   & AN   & AP   & KL   \\ \midrule
Existent & 0.9  & 13.9 & 0.9  & 0.01 \\
Random   & 1    & 16.7 & 0.98 & 0.01 \\
Ones     & 0.75 & 42.5 & 0.75 & 0.01 \\
Zeros    & 0.95 & 14.1 & 0.91 & 0.01 \\
Mean     & 0.91 & 14.1 & 0.91 & 0.01 \\
Median   & 0.95 & 14.0 & 0.91 & 0.01 \\ \bottomrule
\end{tabular}
\end{table}
